# Supplementary material for: Whole-Body Human Kinematics Estimation using Dynamical Inverse Kinematics and Contact-Aided Lie Group Kalman Filter
Source: arXiv:2205.07835 source file (2022-05-16)
Supplement: Supplementary file 1 [file appendix.tex]

\appendix
\label{appendix}
